# Supplementary material for: Efficient Algorithms for Interdicting Facilities in Trees and Bounded Treewidth Graphs
Source: arXiv:2605.27998 source file (2026-05-27)
Supplement: Supplementary file 2 [file Appendix_IP.tex]

\section{IP Formulation}
\label{sec:IP-app}

Similarly to Fröhlich and Ruzika~\cite{FrohlichR22}, we observe that REIC on trees can be formulated as the following integer program, where disconnecting a customer $v \in V\setminus S$ (i.e., setting $x_v=0$) requires that at least one edge $e$ is removed (setting $y_e=1$) on every path from $v$ to a facility $s \in S$. We let $P_{uv}$ denote the unique $u$-$v$ path in $T$.

\begin{equation}\label{eq:ip}\tag{REIC-IP}
\begin{array}{rr@{}llll}
\text{max}&\displaystyle\sum_{v\in V\setminus S} w(v)\,(1-x_v) \\
\text{subject to}& x_v + \displaystyle\sum_{e\in P_{sv}} y_e \ &\geq 1 \quad&\forall v\in V\setminus S, s\in S\\
    &\displaystyle\sum_{e\in E} y_e \ &\leq r\\
    &  x_v \ &\in \{0,1\} \quad&\forall v\in V\setminus S \\
    & y_e \ &\in \{0,1\}\quad&\forall e\in E
\end{array}
\end{equation}

We use the formulation of \ref{eq:ip} in \cref{sec:experimental} and \cref{sec:experimental-app} to compare actual execution times of \myAlgorithm  with those of an integer optimization problem solved using Gurobi.
